# Supplementary material for: Transferable Lindblad Variational Ansatz for Accelerated Steady-State Preparation
Source: arXiv:2611.04919 source file (2026-11-03)
Supplement: Supplementary file 1 [file sm_citation_numbers.tex]

\expandafter\def\csname SMref@verstraete2009\endcsname{1}
\expandafter\def\csname SMurl@verstraete2009\endcsname{https://doi.org/10.1038/nphys1342}
\expandafter\def\csname SMref@diehl2008\endcsname{2}
\expandafter\def\csname SMurl@diehl2008\endcsname{https://doi.org/10.1038/nphys1073}
\expandafter\def\csname SMref@kastoryano2011\endcsname{3}
\expandafter\def\csname SMurl@kastoryano2011\endcsname{https://doi.org/10.1103/PhysRevLett.106.090502}
\expandafter\def\csname SMref@prosen2011\endcsname{4}
\expandafter\def\csname SMurl@prosen2011\endcsname{https://doi.org/10.1103/PhysRevLett.107.137201}
\expandafter\def\csname SMref@znidaric2010\endcsname{5}
\expandafter\def\csname SMurl@znidaric2010\endcsname{https://doi.org/10.1088/1742-5468/2010/05/L05002}
\expandafter\def\csname SMref@landi2022\endcsname{6}
\expandafter\def\csname SMurl@landi2022\endcsname{https://doi.org/10.1103/RevModPhys.94.045006}
\expandafter\def\csname SMref@diehl2010\endcsname{7}
\expandafter\def\csname SMurl@diehl2010\endcsname{https://doi.org/10.1103/PhysRevLett.105.015702}
\expandafter\def\csname SMref@lee2011\endcsname{8}
\expandafter\def\csname SMurl@lee2011\endcsname{https://doi.org/10.1103/PhysRevA.84.031402}
\expandafter\def\csname SMref@sieberer2013\endcsname{9}
\expandafter\def\csname SMurl@sieberer2013\endcsname{https://doi.org/10.1103/PhysRevLett.110.195301}
\expandafter\def\csname SMref@barreiro2011\endcsname{10}
\expandafter\def\csname SMurl@barreiro2011\endcsname{https://doi.org/10.1038/nature09801}
\expandafter\def\csname SMref@schindler2013\endcsname{11}
\expandafter\def\csname SMurl@schindler2013\endcsname{https://doi.org/10.1038/nphys2630}
\expandafter\def\csname SMref@weimer2021\endcsname{12}
\expandafter\def\csname SMurl@weimer2021\endcsname{https://doi.org/10.1103/RevModPhys.93.015008}
\expandafter\def\csname SMref@znidaric2015\endcsname{13}
\expandafter\def\csname SMurl@znidaric2015\endcsname{https://doi.org/10.1103/PhysRevE.92.042143}
\expandafter\def\csname SMref@macieszczak2016\endcsname{14}
\expandafter\def\csname SMurl@macieszczak2016\endcsname{https://doi.org/10.1103/PhysRevLett.116.240404}
\expandafter\def\csname SMref@trotter1959\endcsname{15}
\expandafter\def\csname SMurl@trotter1959\endcsname{https://doi.org/10.1090/S0002-9939-1959-0108732-6}
\expandafter\def\csname SMref@strang1968\endcsname{16}
\expandafter\def\csname SMurl@strang1968\endcsname{https://doi.org/10.1137/0705041}
\expandafter\def\csname SMref@kliesch2011\endcsname{17}
\expandafter\def\csname SMurl@kliesch2011\endcsname{https://doi.org/10.1103/PhysRevLett.107.120501}
\expandafter\def\csname SMref@kraus2008\endcsname{18}
\expandafter\def\csname SMurl@kraus2008\endcsname{https://doi.org/10.1103/PhysRevA.78.042307}
\expandafter\def\csname SMref@carollo2021\endcsname{19}
\expandafter\def\csname SMurl@carollo2021\endcsname{https://doi.org/10.1103/PhysRevLett.127.060401}
\expandafter\def\csname SMref@kochsiek2022\endcsname{20}
\expandafter\def\csname SMurl@kochsiek2022\endcsname{https://doi.org/10.1103/PhysRevA.106.012207}
\expandafter\def\csname SMref@cui2015\endcsname{21}
\expandafter\def\csname SMurl@cui2015\endcsname{https://doi.org/10.1103/PhysRevLett.114.220601}
\expandafter\def\csname SMref@hartmann2019\endcsname{22}
\expandafter\def\csname SMurl@hartmann2019\endcsname{https://doi.org/10.1103/PhysRevLett.122.250502}
\expandafter\def\csname SMref@vicentini2019\endcsname{23}
\expandafter\def\csname SMurl@vicentini2019\endcsname{https://doi.org/10.1103/PhysRevLett.122.250503}
\expandafter\def\csname SMref@farhi2014\endcsname{24}
\expandafter\def\csname SMurl@farhi2014\endcsname{https://arxiv.org/abs/1411.4028}
\expandafter\def\csname SMref@brady2021\endcsname{25}
\expandafter\def\csname SMurl@brady2021\endcsname{https://doi.org/10.1103/PhysRevLett.126.070505}
\expandafter\def\csname SMref@wecker2015\endcsname{26}
\expandafter\def\csname SMurl@wecker2015\endcsname{https://doi.org/10.1103/PhysRevA.92.042303}
\expandafter\def\csname SMref@wiersema2020\endcsname{27}
\expandafter\def\csname SMurl@wiersema2020\endcsname{https://doi.org/10.1103/PRXQuantum.1.020319}
\expandafter\def\csname SMref@martin2022\endcsname{28}
\expandafter\def\csname SMurl@martin2022\endcsname{https://doi.org/10.1103/PhysRevResearch.4.023190}
\expandafter\def\csname SMref@zhou2020\endcsname{29}
\expandafter\def\csname SMurl@zhou2020\endcsname{https://doi.org/10.1103/PhysRevX.10.021067}
\expandafter\def\csname SMref@mbeng2019\endcsname{30}
\expandafter\def\csname SMurl@mbeng2019\endcsname{https://doi.org/10.48550/arXiv.1906.08948}
\expandafter\def\csname SMref@mele2022\endcsname{31}
\expandafter\def\csname SMurl@mele2022\endcsname{https://doi.org/10.1103/PhysRevA.106.L060401}
\expandafter\def\csname SMref@endo2020\endcsname{32}
\expandafter\def\csname SMurl@endo2020\endcsname{https://doi.org/10.1103/PhysRevLett.125.010501}
\expandafter\def\csname SMref@kamakari2022\endcsname{33}
\expandafter\def\csname SMurl@kamakari2022\endcsname{https://doi.org/10.1103/PRXQuantum.3.010320}
\expandafter\def\csname SMref@liu2021\endcsname{34}
\expandafter\def\csname SMurl@liu2021\endcsname{https://doi.org/10.1088/0256-307X/38/8/080301}
\expandafter\def\csname SMref@lindblad1976\endcsname{35}
\expandafter\def\csname SMurl@lindblad1976\endcsname{https://doi.org/10.1007/BF01608499}
\expandafter\def\csname SMref@gks1976\endcsname{36}
\expandafter\def\csname SMurl@gks1976\endcsname{https://doi.org/10.1063/1.522979}
\expandafter\def\csname SMref@lloydviola2001\endcsname{37}
\expandafter\def\csname SMurl@lloydviola2001\endcsname{https://doi.org/10.1103/PhysRevA.65.010101}
\expandafter\def\csname SMref@weimer2010\endcsname{38}
\expandafter\def\csname SMurl@weimer2010\endcsname{https://doi.org/10.1038/nphys1614}
\expandafter\def\csname SMref@dalibard1992\endcsname{39}
\expandafter\def\csname SMurl@dalibard1992\endcsname{https://doi.org/10.1103/PhysRevLett.68.580}
\expandafter\def\csname SMref@dum1992\endcsname{40}
\expandafter\def\csname SMurl@dum1992\endcsname{https://doi.org/10.1103/PhysRevA.45.4879}
\expandafter\def\csname SMref@stinespring1955\endcsname{41}
\expandafter\def\csname SMurl@stinespring1955\endcsname{https://doi.org/10.1090/S0002-9939-1955-0069403-4}
\expandafter\def\csname SMref@wang2013channels\endcsname{42}
\expandafter\def\csname SMurl@wang2013channels\endcsname{https://doi.org/10.1103/PhysRevLett.111.130504}
\expandafter\def\csname SMref@sweke2014\endcsname{43}
\expandafter\def\csname SMurl@sweke2014\endcsname{https://doi.org/10.1103/PhysRevA.90.022331}
\expandafter\def\csname SMref@dive2015\endcsname{44}
\expandafter\def\csname SMurl@dive2015\endcsname{https://doi.org/10.1103/PhysRevA.92.032111}
\expandafter\def\csname SMref@jozsa1994\endcsname{45}
\expandafter\def\csname SMurl@jozsa1994\endcsname{https://doi.org/10.1080/09500349414552171}
\expandafter\def\csname SMref@fuchs1999\endcsname{46}
\expandafter\def\csname SMurl@fuchs1999\endcsname{https://doi.org/10.1109/18.761271}
\expandafter\def\csname SMref@byrd1995\endcsname{47}
\expandafter\def\csname SMurl@byrd1995\endcsname{https://doi.org/10.1137/0916069}
\expandafter\def\csname SMref@grant2019\endcsname{48}
\expandafter\def\csname SMurl@grant2019\endcsname{https://doi.org/10.22331/q-2019-12-09-214}
\expandafter\def\csname SMref@skolik2021\endcsname{49}
\expandafter\def\csname SMurl@skolik2021\endcsname{https://doi.org/10.1007/s42484-020-00036-4}
\expandafter\def\csname SMref@puig2025\endcsname{50}
\expandafter\def\csname SMurl@puig2025\endcsname{https://doi.org/10.1103/PRXQuantum.6.010317}
\expandafter\def\csname SMref@preskill2018\endcsname{51}
\expandafter\def\csname SMurl@preskill2018\endcsname{https://doi.org/10.22331/q-2018-08-06-79}
\expandafter\def\csname SMref@cerezo2021review\endcsname{52}
\expandafter\def\csname SMurl@cerezo2021review\endcsname{https://doi.org/10.1038/s42254-021-00348-9}
\expandafter\def\csname SMref@poulin2010\endcsname{54}
\expandafter\def\csname SMurl@poulin2010\endcsname{https://doi.org/10.1103/PhysRevLett.104.190401}
\expandafter\def\csname SMref@barthel2012\endcsname{55}
\expandafter\def\csname SMurl@barthel2012\endcsname{https://doi.org/10.1103/PhysRevLett.108.230504}
\expandafter\def\csname SMref@kastoryanotemme2013\endcsname{56}
\expandafter\def\csname SMurl@kastoryanotemme2013\endcsname{https://doi.org/10.1063/1.4804995}
\expandafter\def\csname SMref@minganti2018\endcsname{57}
\expandafter\def\csname SMurl@minganti2018\endcsname{https://doi.org/10.1103/PhysRevA.98.042118}
\expandafter\def\csname SMref@suzuki1976\endcsname{58}
\expandafter\def\csname SMurl@suzuki1976\endcsname{https://doi.org/10.1007/BF01609348}
\expandafter\def\csname SMref@childsli2017\endcsname{59}
\expandafter\def\csname SMurl@childsli2017\endcsname{https://doi.org/10.26421/QIC17.11-12-1}
\expandafter\def\csname SMref@clevewang2017\endcsname{60}
\expandafter\def\csname SMurl@clevewang2017\endcsname{https://doi.org/10.4230/LIPIcs.ICALP.2017.17}
\expandafter\def\csname SMref@verstraete2004\endcsname{61}
\expandafter\def\csname SMurl@verstraete2004\endcsname{https://doi.org/10.1103/PhysRevLett.93.207204}
\expandafter\def\csname SMref@zwolak2004\endcsname{62}
\expandafter\def\csname SMurl@zwolak2004\endcsname{https://doi.org/10.1103/PhysRevLett.93.207205}
\expandafter\def\csname SMref@werner2016\endcsname{63}
\expandafter\def\csname SMurl@werner2016\endcsname{https://doi.org/10.1103/PhysRevLett.116.237201}
\expandafter\def\csname SMref@park2024\endcsname{64}
\expandafter\def\csname SMurl@park2024\endcsname{https://doi.org/10.22331/q-2024-02-01-1239}
\expandafter\def\csname SMref@huang2020\endcsname{65}
\expandafter\def\csname SMurl@huang2020\endcsname{https://doi.org/10.1038/s41567-020-0932-7}
\expandafter\def\csname SMref@elben2023\endcsname{66}
\expandafter\def\csname SMurl@elben2023\endcsname{https://doi.org/10.1038/s42254-022-00535-2}
\expandafter\def\csname SMref@elben2018\endcsname{67}
\expandafter\def\csname SMurl@elben2018\endcsname{https://doi.org/10.1103/PhysRevLett.120.050406}
\expandafter\def\csname SMref@brydges2019\endcsname{68}
\expandafter\def\csname SMurl@brydges2019\endcsname{https://doi.org/10.1126/science.aau4963}
\expandafter\def\csname SMref@schuld2019\endcsname{69}
\expandafter\def\csname SMurl@schuld2019\endcsname{https://doi.org/10.1103/PhysRevA.99.032331}
\expandafter\def\csname SMref@wierichs2022\endcsname{70}
\expandafter\def\csname SMurl@wierichs2022\endcsname{https://doi.org/10.22331/q-2022-03-30-677}
\expandafter\def\csname SMref@banchi2021\endcsname{71}
\expandafter\def\csname SMurl@banchi2021\endcsname{https://doi.org/10.22331/q-2021-01-25-386}
\expandafter\def\csname SMref@spall1992\endcsname{72}
\expandafter\def\csname SMurl@spall1992\endcsname{https://doi.org/10.1109/9.119632}
\expandafter\def\csname SMref@mcclean2018\endcsname{73}
\expandafter\def\csname SMurl@mcclean2018\endcsname{https://doi.org/10.1038/s41467-018-07090-4}
\expandafter\def\csname SMref@cerezo2021cost\endcsname{74}
\expandafter\def\csname SMurl@cerezo2021cost\endcsname{https://doi.org/10.1038/s41467-021-21728-w}
\expandafter\def\csname SMref@wang2021\endcsname{75}
\expandafter\def\csname SMurl@wang2021\endcsname{https://doi.org/10.1038/s41467-021-27045-6}
\expandafter\def\csname SMref@stokes2020\endcsname{76}
\expandafter\def\csname SMurl@stokes2020\endcsname{https://doi.org/10.22331/q-2020-05-25-269}
\expandafter\def\csname SMref@cutoff2012\endcsname{77}
\expandafter\def\csname SMurl@cutoff2012\endcsname{https://doi.org/10.1088/1751-8113/45/7/075307}
\expandafter\def\csname SMref@lva_data_code\endcsname{53}
\expandafter\def\csname SMurl@lva_data_code\endcsname{https://github.com/yunzhuofan/Transferable-Lindblad-Variational-Ansatz-for-Accelerated-Steady-State-Preparation}
